# Supplementary material for: On Central Primitives for Quantum Cryptography with Classical Communication
Source: arXiv:2402.17715 source file (2024-06-28)
Supplement: Supplementary file 1 [file appendix.tex]

%eprint
\appendix

\section{Proofs and definitions for $\EVOWP$ from QCCC primitives}\label{app:ev-from-qcc}

\section{Proofs for $\OWP$ Amplification, Combiners, and Universal
Constructions}\label{app:amp-comb-univ}

\subsection{Amplification}

\section{Proofs for $\OWP$ security amplification}\label{app:sec-amp}
